# Supplementary material for: Multi-Bit Distortion-Free Watermarking for Large Language Models
Source: arXiv:2402.16578 source file (2024-02-26)
Supplement: Supplementary file 1 [file appendix.tex]

% \documentclass[11pt]{article}
% \usepackage{appendix}

% \usepackage{latexsym}
% \usepackage{amsfonts}
% \usepackage{amsmath}
% \usepackage{algpseudocode}
% \usepackage{algorithm}
% \usepackage{fullpage}
% \usepackage{graphicx}
% \newcommand{\N}{\mathcal{N}}
% \newcommand{\R}{\mathcal{R}}
% \newcommand{\A}{\mathcal{A}}

%\algnewcommand\algorithmicforeach{\textbf{for each}}
%\algdef{S}[FOR]{ForEach}[1]{\algorithmicforeach\ #1\ \algorithmicdo}
%\algrenewcommand\algorithmicrequire{\textbf{Input:}}
%\algrenewcommand\algorithmicensure{\textbf{Output:}}
%\let\oldReturn\Return
%\renewcommand{\Return}{\State\oldReturn}
% \begin{document}

\section{Lower Bound on the Required Number of Tokens in \cite{Aaronson2023}.}

Using their scoring metric, let $S_{W}$ denote the summation of score for a watermarked text with $L$ tokens in response to prompt $\alpha$, while $S_{NW}$ is the summation of score for a non-watermarked text with $L$ tokens. According to \cite{Aaronson2023}, 

\begin{equation}
\begin{aligned}
    &S_{NW}\xrightarrow{d}\mathcal{N}(L, L)\\
    &S_{W}\xrightarrow{d}\mathcal{N}(L+(\frac{\pi^{2}}{6}-1)\zeta(\alpha) L, \frac{\pi^{2}}{6}L)
\end{aligned}
\end{equation}

Let FPR=FNR=$\eta$ which is the misclassification probability that is acceptable, and $\theta$ is the threshold which is compared with the summation of score. The ideal watermark detector should ensure:

\begin{equation}
    \begin{aligned}
        \Pr[S_{W}&\leq\theta]\leq\eta\\
        \Pr[S_{NW}&\geq\theta]\leq\eta
    \end{aligned}
\end{equation}

Since 

\begin{equation}
    \begin{aligned}
       \Pr[S_{W}\leq\theta]&=1-Q(\frac{\theta-(L+(\frac{\pi^{2}}{6}-1)\zeta(\alpha) L)}{\sqrt{\frac{\pi^{2}}{6}L}})\\
       &=Q(\frac{(L+(\frac{\pi^{2}}{6}-1)\zeta(\alpha) L-\theta}{\sqrt{\frac{\pi^{2}}{6}L}})\\
       &\leq \frac{1}{2}exp(-\frac{((L+(\frac{\pi^{2}}{6}-1)\zeta(\alpha) L-\theta)^{2}}{\frac{\pi^{2}}{3}L})
    \end{aligned}
\end{equation}

Therefore

\begin{equation}
    \begin{aligned}
        \frac{1}{2}exp(-\frac{((L+(\frac{\pi^{2}}{6}-1)\zeta(\alpha) L-\theta)^{2}}{\frac{\pi^{2}}{3}L})\leq\eta
    \end{aligned}
\end{equation}

\begin{equation}\label{deriveLmin}
    \begin{aligned}
        L+(\frac{\pi^{2}}{6}-1)\zeta(\alpha) L-\theta)^{2}\geq\frac{\pi^{2}}{3}L\gamma
    \end{aligned}
\end{equation}
where $\gamma=ln\frac{1}{2\eta}$.

From $\Pr[S_{NW}\geq\theta]\leq\eta$

\begin{equation}
    \begin{aligned}
        \Pr[S_{NW}\geq\theta]=Q(\frac{\theta-L}{\sqrt{L}})\leq\frac{1}{2}exp(-\frac{(\theta-L)^{2}}{2L})
    \end{aligned}
\end{equation}

Therefore, 

\begin{equation}
    \begin{aligned}
        \Pr[S_{NW}\geq\theta]=Q(\frac{\theta-L}{\sqrt{L}})\leq\frac{1}{2}exp(-\frac{(\theta-L)^{2}}{2L})
    \end{aligned}
\end{equation}

So, $\theta\in[L-\sqrt{2L\gamma}, L+\sqrt{2L\gamma}]$.

To derive the minimum $L$ from eq. (\ref{deriveLmin}), $\theta=L+\sqrt{2L\gamma}$ is put in it, and thus
\begin{equation}
    \begin{aligned}
        L_{min}=\frac{2+\frac{\pi^{2}}{3}+4\sqrt{\frac{\pi^{2}}{6}}}{\zeta(\alpha)^{2}}\gamma
    \end{aligned}
\end{equation}

Thus, $L_{min}=O(\frac{1}{\zeta(\alpha)^{2}}\ln\frac{1}{\eta})$.

% \bibliography{bibliograpgy}
% \end{document}
